# Supplementary material for: Competing Ferri- and Antiferromagnetic Phases in Geometrically Frustrated LuFe2O4
Source: arXiv:1111.0746 ancillary file (2011-11-03)
Supplement: Supplementary file 1 [file supplementary_info.pdf]

## Supplementary Information to:
## "Competing Ferri- and Antiferromagnetic Phases in Geometrical Frustrated $LuFe_2O_4$"

**Authors:** J. de Groot, K. Marty, M. D. Lumsden, A. D. Christianson, S. E. Nagler, S. Adiga, W. J. H. Borghols, K. Schmalzl, Z. Yamani, S. R. Bland, R. de Souza, W. Schweika, Y.Su, and M. Angst

In this supplement we provide additional details of our spin structures determination in the 6× larger $C2/m$ charge ordered cell (see Figs. S1 and S2 and [4]), which corresponds, according to all observed magnetic reflections, to the magnetic cell for one domain (it is clear from the location of the reflections that there are three domains [1]). We will explain how the spin structures for both magnetic phases were determined in this new cell. This supplement closes with a consideration of why these solutions can not be obtained by standard representation analysis.

# Magnetic Cell and Approach

From symmetry analysis of the charge order in the high-temperature hexagonal cell [5], two irreducible representations are allowed for each domain (Fig. S2), both of which lower the space group to $C2/m$. These two representations correspond to different origin positions (i.e. center of inversion) in the monoclinic cell (Fig. S2). In one case the center of inversion is at the Lu positions between the bilayers and for the other case the inversion center is located between the two Fe-layers of a particular bilayer. However, the cell origin has no influence on the refinement result.

For tiny deviations in the Fe-position in Tab. I only small differences upon refinement are observed. The transformation rules, which describe the $(h, k, \ell)$-relationship between the hexagonal cell and the monoclinic domains, is presented in Tab. II. For comparison with previous work, we will use hexagonal notation for indexing the reflections, unless noted otherwise.

Rather than starting with a limited number of candidate spin structures from representation analysis, we considered all Ising spin structures having the periodicity of the observed magnetic cell. Very broad-sized restrictions based on experimental data from four types of magnetic reflections are used to limit these possible structures to a small set of feasible ones. These remaining solutions are then refined against experimental data.

TABLE I: Half of the Fe-sites which are used for the spin refinement. The other half is obtained by adding $(\frac{1}{2}\,\frac{1}{2}\,0)$ (C-centering) to the here presented positions. The here presented atomic positions are from symmetry analysis of the charge order in the hexagonal high-temperature cell.

| | $p_{ix}$ | $p_{iy}$ | $p_{iz}$ | Wyck. site | | $p_{ix}$ | $p_{iy}$ | $p_{iz}$ | Wyck. site |
|---|---|---|---|---|---|---|---|---|---|
| Fe1 | 0.8598 | 0.833 | 0.0721 | $8j_1$ | Fe7 | 0.8566 | 0.0 | 0.5721 | $4i_2$ |
| Fe2 | 0.8598 | 0.5 | 0.0721 | $4i_1$ | Fe8 | 0.8566 | 0.666 | 0.5721 | $8j_2$ |
| Fe3 | 0.8598 | 0.166 | 0.0721 | $8j_1$ | Fe9 | 0.8566 | 0.333 | 0.5721 | $8j_2$ |
| Fe4 | 0.6434 | 0.833 | 0.4269 | $8j_2$ | Fe10 | 0.6402 | 0.0 | 0.9269 | $4i_1$ |
| Fe5 | 0.6434 | 0.5 | 0.4269 | $4i_2$ | Fe11 | 0.6402 | 0.666 | 0.9269 | $8j_1$ |
| Fe6 | 0.6434 | 0.166 | 0.4269 | $8j_2$ | Fe12 | 0.6402 | 0.333 | 0.9269 | $8j_1$ |

This $C2/m$ cell contains 2×12 Fe-atoms (see Tab. I). The C-centering condition is preserved also for spin order in both magnetic phases, otherwise additional magnetic reflection would appear, which are absent in all our observations. Most generally, the spin configuration is therefore specified by the spins on 12 Fe-atoms. We considered all possible spin configurations by ignoring symmetry other than the C-centering and using Ising spins $||c_{\text{hex}}$ ($\perp\vec{a}$ and $\perp\vec{b}$ in the monoclinic cell). The direction of the Ising spin at site $a_i$ is represented by either spin up or down $a_i = (1, -1)$. For completeness we also considered partial disorder of magnetic moments (sites with $a_i = 0$). We started the simulation by using equal magnetic moments for $Fe^{2+}$ and $Fe^{3+}$, which should be a good approximation given the strong orbital magnetic component for the $Fe^{2+}$ ions [2, 3] with slightly lower spin. We also implemented slightly different moments for $Fe^{2+}$ and $Fe^{3+}$. This magnetic contrast will give relative small changes in the reflection patterns and is thus not affecting the determination of candidates spin structures described in the two paragraphs below (the resulting $\chi^2$ upon refinement will change only slightly). The intensity (apart from a correction by form, polarization and Debey-Waller factor) for each allowed $(h+k = 2n)$ reflection in this monoclinic cell is $I(hk\ell) \sim |F_{hk\ell}|^2$ with $F_{hk\ell} = \sum_{j=1}^{12} a_j \cdot e^{i(p_{jx}\cdot h + p_{jy}\cdot k + p_{jz}\cdot \ell)}$, where $h$, $k$ and $\ell$ are coordinates of the reciprocal monoclinic cell. The total amount of $3^{12}$=531441 possible spin structures is too big for refining them all. To narrow the number of candidates to a tractable number we compared relative intensities on different magnetic reflections with intensity restrictions to exclude solutions obviously not matching our observations. These restrictions were very broad-sized

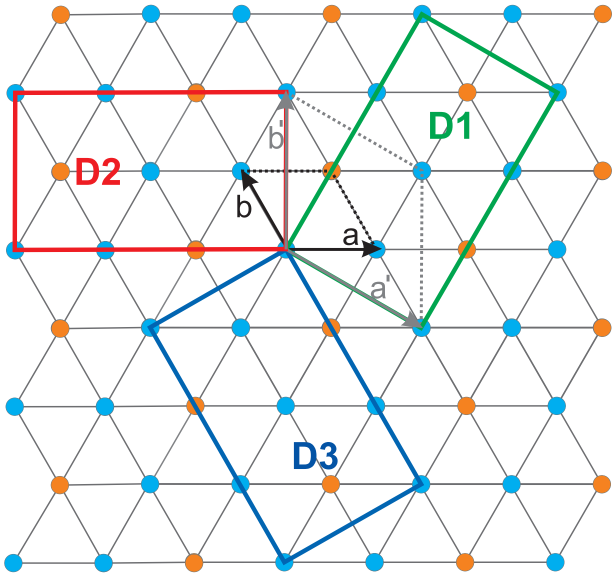


FIG. S1: Transformation between the hexagonal cell (black) and the three monoclinic domains (D1, D2 and D3) in the $a, b$-plane.

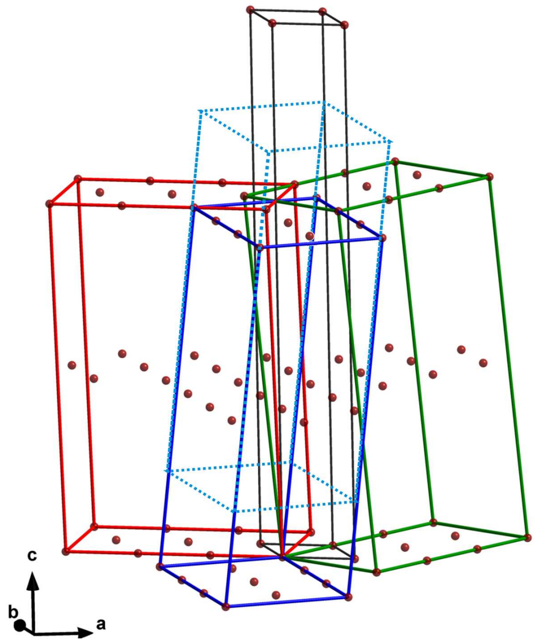


FIG. S2: Relation between the hexagonal lattice and the three monoclinic domains (showing only Lu Atoms). The final domains positions are achieved by shifting them by 1/4 along the $c$ lattice direction, as indicated for the domain D3 by dotted lines, the others are omitted for clarity.

to account for uncertainty e.g. in the Debye-Waller factor. Except where noted, the restrictions are completely independent of domain populations. This approach was done for the two magnetic phases yielding different intensities on magnetic reflections. The remaining structures were analyzed for symmetry equivalent structures shifted by $(0, 0, \frac{1}{2})$ or $\pm(0, 0.333, 0)$ with respect to the unit cell or with all spin directions reversed. Assuming no $Fe^{2+/3+}$ contrast, these equivalent structures are indistinguishable in diffraction and equivalent with regards to symmetry. The final spin structures shown in Fig. 1b/c are determined only up to this equivalence, althouh magnetic contrast was also considered (see later).

TABLE II: Transformation rules for the $(h, k, \ell)$ between the hexagonal and monoclinic unit cell ($\beta = 97.72°$) with its three different domains $D1$, $D2$ and $D3$.

| | $D1$ | $D2$ | $D3$ |
|---|---|---|---|
| $h_{mon}=$ | $h_{hex} - k_{hex}$ | $3(h_{hex} + k_{hex})$ | $-4h_{hex} - 2k_{hex}$ |
| $k_{mon}=$ | $3(h_{hex} + k_{hex})$ | $-4h_{hex} - 2k_{hex}$ | $h_{hex} - k_{hex}$ |
| $\ell_{mon}=$ | $\frac{1}{3}(-h_{hex} + k_{hex} - 2\ell_{hex})$ | $\frac{1}{3}(-h_{hex} + k_{hex} - 2\ell_{hex})$ | $\frac{1}{3}(-h_{hex} + k_{hex} - 2\ell_{hex})$ |

# Restrictions and refinement for the low-$H$ phase

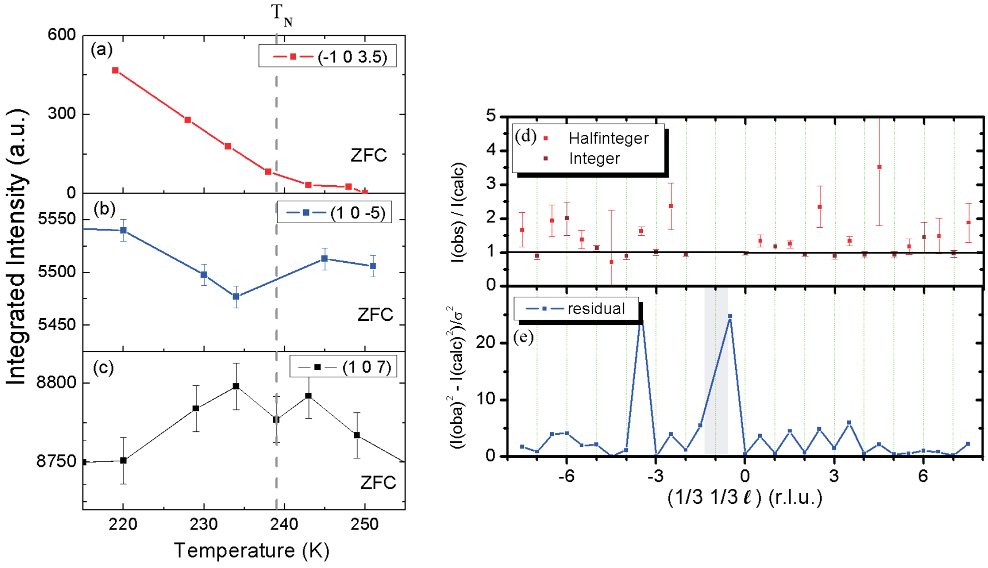


FIG. S3: (a-c) Temperature dependences of the integrated intensity for different types of reflection $(\bar{1}0\frac{7}{2})$ (a), $(10\bar{5})$ (b) and (107) (c) (d). Ratio between observation and model (AFM spin structure shown in Fig. 1c) for integer and halfinteger $(\frac{1}{3},\frac{1}{3},\ell)$ reflections in the low-$H$ phase. (e) Residual $\chi^2$ contributions between model and observation for each reflection in the AFM spin structure. The gray area indicates the magnet dark angle. The reflection $(\frac{1}{3},\frac{1}{3},-\frac{7}{2})$ was excluded due to an overlap with the (006) reflection from a small second grain.

Comparing all measured integrated intensities (see Tab. III) with our calculated intensities some broad size restrictions for the low-$H$ phase solution can be made. Note that all reflections are indexed in $R\bar{3}m$ (hexagonal setting) crystallographic cell:

- The first set of restrictions suppresses spin structures which have no similar relative intensities on the $I(\frac{1}{3},\frac{1}{3},\text{integer})$ as in [1]. Herefore the following conditions are used: $5.5 < I(\frac{1}{3},\frac{1}{3},3) < 6.5$ and $0.8 < I(\frac{1}{3},\frac{1}{3},6) < 1.2$ (all normalized on $I(\frac{1}{3},\frac{1}{3},0) = 16$). Afterwards ∼15000 structures remain, which need to be checked, many of them having exactly the same relative intensity on the $(\frac{1}{3},\frac{1}{3},\ell)$-line.

- Comparing different $(00\frac{3}{2})$-type reflections according to Tab. III, the following restriction can be made: $2\cdot I(\bar{1}\,0\,\frac{1}{2}) < I(\bar{1}\,0\,\frac{7}{2}) < 5\cdot I(\bar{1}\,0\,\frac{1}{2})$ and from Fig. 3b it is clear that both reflections should have intensities $>0$; afterwards $\sim 3800$ solutions remain.

- A third restriction compares the integrated intensity from one of the $(00\frac{3}{2})$-type reflection with the $(\frac{1}{3}\frac{1}{3}0)$ reflection as follows: $I(\bar{1}\,0\,\frac{7}{2}) < I(\frac{1}{3}\frac{1}{3}0)$. Here, the width of the condition was chosen very broad. According to the domain structure of $LuFe_2O_4$ we took also into account that the $(00\frac{3}{2})$-type reflections originate from all three domains in contrast to the $(\frac{1}{3}\frac{1}{3}\ell)$-type reflections which originate from a single domain. This condition is valid for any domain population, even the extreme case of only one domain present. This restriction reduces the number of possible solutions to $\sim 1700$.

- Setting only upper limits for the $(\frac{1}{3},\frac{1}{3},\text{halfinteger})$ type reflections according to Tab. III as following: $I(\frac{1}{3},\frac{1}{3},\frac{3}{2}) < 8$, $I(\frac{1}{3},\frac{1}{3},\frac{9}{2}) < 3$ and $I(\frac{1}{3},\frac{1}{3},\frac{15}{2}) < 6$. To account for the possibility that the observed intensity on $(\frac{1}{3},\frac{1}{3},\text{halfinteger})$ types originates from cross-contamination from the high-$H$ phase, this restriction also allows for no intensity on this reflections. The total amount of possible solutions is reduced to 252 by this condition.

- The temperature-dependence through the Néel-temperature (in $H=0$) of two structural Bragg-reflections indicate no systematic increase below $T_N$, suggesting any magnetic contribution to be small (see Fig. S3b/c; the error bars shown, resulting from fits of rocking curves, obviously underestimate the real error). From the sensitivity of the measurement we establish upper limits for possible magnetic contributions; normalized to $I(\frac{1}{3},\frac{1}{3},0) = 16$

the condition is $I(107) < 5$ and $I(10\overline{5}) < 5$. The value of 5 for both structural reflections takes into account that it originates from all three domains and this reflections have a large $Q$-value. This condition leaves 168 solutions corresponding to 7 symmetry inequivalent structures, of which only one is fully ordered (see Tab. IV).

TABLE III: Measured integrated intensities in the low-$H$ phase on several reflections (indexed in the $R\overline{3}m$ hexagonal cell) at different temperatures, measured by non-polarized neutron diffraction.

| hkl (hex) | hkl (mono) | Integrated Intensity | $Q(\text{Å}^{-1})$ | Temperature (K) |
|---|---|---|---|---|
| $(\frac{1}{3}\,\frac{1}{3}\,0)$ | $(0\,2\,0)$ | 1470 | 1.22 | 220 |
| $(\overline{1}\,0\,\frac{1}{2})$ | $(\overline{1}\,\overline{3}\,0)$ | 154 | 2.11 | 220 |
| $(\overline{1}\,0\,\frac{7}{2})$ | $(\overline{1}\,\overline{3}\,\overline{2})$ | 452 | 2.28 | 220 |
| $(\frac{1}{3}\,\frac{1}{3}\,\frac{3}{2})$ | $(0\,2\,\overline{1})$ | 601 | 1.27 | 220 |
| $(\frac{1}{3}\,\frac{1}{3}\,3)$ | $(0\,2\,\overline{2})$ | 577.6 | 1.43 | 220 |
| $(\frac{1}{3}\,\frac{1}{3}\,\frac{9}{2})$ | $(0\,2\,\overline{3})$ | 95.4 | 1.65 | 220 |
| $(\frac{1}{3}\,\frac{1}{3}\,6)$ | $(0\,2\,\overline{4})$ | 97.3 | 1.92 | 220 |
| $(\frac{1}{3}\,\frac{1}{3}\,\frac{15}{2})$ | $(0\,2\,\overline{5})$ | 77.2 | 2.23 | 220 |
| $(1\,0\,\overline{5})^a$ | $(1\,3\,3)$ | $\leq$150 | 2.45 | 190 |
| $(1\,0\,7)^a$ | $(1\,3\,\overline{5})$ | $\leq$150 | 2.73 | 190 |

[a]magnetic contribution

The remaining solutions exhibit different intensity contributions for integer and halfinteger $\ell$ along the $(\frac{1}{3}\frac{1}{3}\ell)$-line. A refinement as in [1], but including both $(\frac{1}{3}, \frac{1}{3}$,integer) and $(\frac{1}{3}, \frac{1}{3}$,halfinteger) reflections can decide between those. Before starting refinement some reflections need to be excluded due to uncertain conditions in their measurement. An additional neutron diffraction measurement suggests an overlap of $(\frac{1}{3}, \frac{1}{3}, -\frac{7}{2})$ with the (006)-structural reflection of a small second grain, which puts the experimental intensity on this reflection in doubt. The reflections $(\frac{1}{3}, \frac{1}{3}, -\frac{1}{2})$ and $(\frac{1}{3}, \frac{1}{3}, -\frac{3}{2})$ as likely affected by the magnet dark angle are excluded as well. The charge order superstructure contributes to weak additional (non-magnetic) intensity on the $(\frac{1}{3}, \frac{1}{3}$,halfinteger) reflections. As x-ray diffraction suggests, no large changes on this charge order reflection intensity [5] is observed on cooling, this could be taken into account as a good approximation by subtracting the intensities measured at 280 K.

To determine the right spin structure for the low-$H$ phase a refinement similar to the one in [1] was thus conducted, and only one of the 7 spin structures, no. 1 in Tab. IV (also the only fully ordered one) has an at least moderately good reduced $\chi^2$=2.15. The strong deviation between observed and measured intensity on reflections excluded before the refinement would give a strong contribution ($\sim +1.7$) to the reduced $\chi^2$ (see Fig. S3e) confirming their exemption.

Too much observed intensity on $(\frac{1}{3}, \frac{1}{3}$,halfinteger) is readily identified (see Fig. S3d) as the largest contribution to the reduced $\chi^2$ from the correct low-$H$ solution. We considered two possible effects influencing the $(\frac{1}{3}, \frac{1}{3}$,halfinteger) reflections:

i) As suggested in [1], intensity could be contributed by the $Fe^{2+/3+}$ magnetic contrast. Most charge configurations, e.g. the CO proposed in [5, 6] do not give any significant change in the refinement for acceptable $Fe^{2+}$ moments, though for an alternative CO with charged bilayers (considered in [5], but appraised as physically unlikely) a further improvement of $\chi^2$ to $\sim$1 is observed. We note that corresponding simulations with $Fe^{2+}/Fe^{3+}$ magnetic contrast were also carried out for the other spin structures, but any improvements were always small compared to large differences in $\chi^2$ for solution 1 (see Tab. IV).

ii) Due to the fact that the solution for the high-$H$ phase has its strongest intensity contribution on the $(\frac{1}{3}, \frac{1}{3}$,halfinteger) reflections, which have among themselves the same relative intensities as in the low-$H$ phase (see below); cross contamination could at least partially explain the systematically higher observed intensity on $(\frac{1}{3}, \frac{1}{3}$,halfinteger) reflections compared to the model (see Fig. S3d). By refining the $(\frac{1}{3}, \frac{1}{3}$,halfinteger) with a scale factor a too high intensity of $\sim$40% on this type of reflection could be identified, which would correspond to a cross contamination of $\sim$15% from the high-$H$ phase. The necessary 15% contamination would give a considerably larger remanent magnetization than the observed 5% in Fig. 3b. Cross contamination alone can therefore not explain all the improvement in $\chi^2$.

Both corrections may contribute to enhanced intensity on $(\frac{1}{3}, \frac{1}{3}$,halfinteger) type reflections. We can therefore not quantify the relative contribution.

TABLE IV: Possible spin structures for the low-$H$ phase obtained from our simulations explained in the text. Only half of the spins on the particular Fe-sites according to Tab. III are presented. The other half is obtained by adding $(\frac{1}{2}\,\frac{1}{2}\,0)$ with the same spin direction due to the still valid C-centering condition.

| low-$H$ solution ($\chi^2$): | Fe1 | Fe2 | Fe3 | Fe4 | Fe5 | Fe6 | Fe7 | Fe8 | Fe9 | Fe10 | Fe11 | Fe12 |
|---|---|---|---|---|---|---|---|---|---|---|---|---|
| 1 (2.15) | ↑ | ↓ | ↑ | ↑ | ↓ | ↓ | ↓ | ↓ | ↑ | ↓ | ↑ | ↑ |
| 2 (15.79) | ↓ | ↓ | 0 | 0 | 0 | ↑ | ↓ | ↑ | ↓ | ↓ | ↑ | ↓ |
| 3 (18.01) | ↓ | ↓ | 0 | 0 | 0 | ↑ | ↓ | ↑ | 0 | ↓ | ↑ | 0 |
| 4 (17.07) | ↓ | ↓ | 0 | ↑ | 0 | ↑ | ↓ | ↑ | 0 | ↓ | ↑ | ↓ |
| 5 (12.31) | ↓ | ↓ | ↑ | ↓ | 0 | ↑ | 0 | ↑ | ↓ | ↓ | ↑ | ↓ |
| 6 (10.45) | ↓ | ↓ | ↑ | 0 | 0 | ↑ | 0 | ↑ | 0 | ↓ | ↑ | ↓ |
| 7 (8.95) | ↓ | 0 | ↑ | ↓ | 0 | 0 | 0 | 0 | ↓ | 0 | ↑ | ↓ |

## Restrictions and refinement for the high-$H$ phase

Measured intensities for the high-$H$ phase are given in Tab. V. Interestingly, the ratio of the intensities for different $(\frac{1}{3},\frac{1}{3}$,halfinteger) reflections remain the same for both phases. Only an overall factor changes the absolute intensities (all increase with applied field). The same is true for $(\frac{1}{3},\frac{1}{3}$,integer) reflections, except that all intensities decrease with applied field. The $(\frac{1}{3},\frac{1}{3}$,integer) reflections could in principle be a cross-contamination from the low-$H$ phase. We therefore do not use lower-limit conditions for these, although Fig. 3b suggests an only modest cross-contamination of possibly 12% when it is applied after zero-field cooling; for field-cooling it is likely considerable lower.

- Comparing all $(\frac{1}{3}\frac{1}{3}\ell)$ with $\ell$ integer and halfinteger values according to the observed in-field neutron-diffraction pattern and allowing for cross contamination from the AFM-phase $\sim$1400 possibilities remain. Conditions: $I(\frac{1}{3},\frac{1}{3},0) < 9.5$, $I(\frac{1}{3},\frac{1}{3},3) < 8$, $I(\frac{1}{3},\frac{1}{3},\frac{9}{2}) < 8$ and $I(\frac{1}{3},\frac{1}{3},6) < 4$. All intensities are normalized to $I(\frac{1}{3},\frac{1}{3},\frac{3}{2}) = 16$ reflection; the most intense in this phase.
- The $(\bar{1}02)$+$(00\frac{3}{2})$ reflection is strongly suppressed (by $\sim$85%) in the high-$H$ phase. The small intensity remaining is likely due to cross-contamination. For considering this we only set an upper limit for the reflection: $I(\bar{1}\,0\,\frac{7}{2}) < \frac{1}{10}\cdot I(\frac{1}{3}\frac{1}{3}\frac{3}{2})$ and $I(\bar{1}\,0\,\frac{1}{2}) < \frac{1}{10}\cdot I(\frac{1}{3}\frac{1}{3}\frac{3}{2})$. This was done by taking into account again that the $(\frac{1}{3}\frac{1}{3}\frac{3}{2})$ originates from one domain as above. This restriction reduces the possible solutions to 72.
- After comparing the magnetic contribution on top of different structural reflections: $I(10\bar{5}) < 9.5$ and $I(107) < 9.5$, only 26 solutions remain, corresponding to 3 symmetry inequivalent ones, listed in Tab. VI. Similar to the low-$H$ phase only one of these solutions is fully ordered.

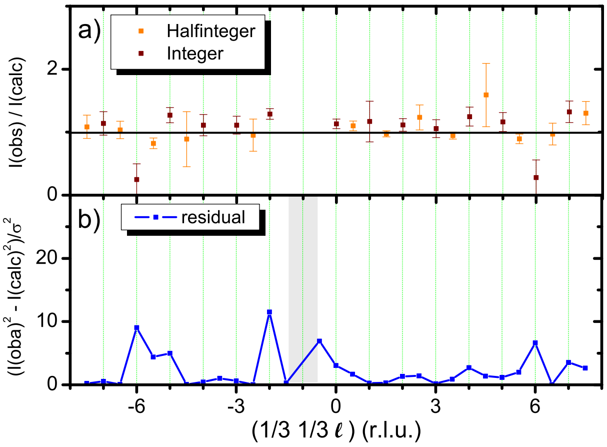


FIG. S4: (a) Deviation between model and observation for both integer and halfinteger $(\frac{1}{3},\frac{1}{3},\ell)$ reflections in the fully ordered fM spin structure. (b) Residual $\chi^2$ contribution between model and observations for each reflection in the full ordered fM spin structure. The gray area indicates the magnet dark angle. The reflection $(\frac{1}{3},\frac{1}{3},-\frac{7}{2})$ was excluded due to an overlap with the (006) reflection from a small second grain.

As for the low-$H$ phase above, the 3 remaining structures were refined against experimental data, in this case obtained at 220 K and 2.5 T after field cooling. Only the fully-ordered structure No. 1 in Tab. VI has a reasonable reduced

$\chi^2$=2.05 (after excluding the same reflections as in the low-$H$ phase). Too much observed intensity on ($\frac{1}{3}$, $\frac{1}{3}$,integer) is readily identified (see Fig. S3) as the largest contribution to the reduced $\chi^2$ from the correct high-$H$ solution. As for the low-$H$ phase the refinement can be improved by taking into account a small cross-contamination by the low-$H$ phase or different $Fe^{2+}$ moments following the rejected CO presented in [5] (again the reduced $\chi^2$ did not improve with other CO configurations). A small cross contamination of about ∼6% gives similar reduced $\chi^2$, making it difficult to argue what the right correction is, similar to the low-$H$ phase.

TABLE V: Measured integrated intensities in the high-$H$ phase on several reflections (indexed in the $R\bar{3}m$ hexagonal cell) at different temperatures, measured by non-polarized neutron diffraction.

| hkl (hex) | hkl (mono) | Integrated Intensity | $Q$(Å$^{-1}$) | Temperature (K) |
|---|---|---|---|---|
| $(\frac{1}{3}\,\frac{1}{3}\,0)$ | $(0\,2\,0)$ | 899 | 1.22 | 220 |
| $(\bar{1}\,0\,\frac{1}{2})$ | $(\bar{1}\,\bar{3}\,0)$ | 22.5 | 2.11 | 220 |
| $(\bar{1}\,0\,\frac{7}{2})$ | $(\bar{1}\,\bar{3}\,\bar{2})$ | 69 | 2.28 | 220 |
| $(\frac{1}{3}\,\frac{1}{3}\,\frac{3}{2})$ | $(0\,2\,\bar{1})$ | 1540 | 1.27 | 220 |
| $(\frac{1}{3}\,\frac{1}{3}\,3)$ | $(0\,2\,\bar{2})$ | 577.6 | 1.43 | 220 |
| $(\frac{1}{3}\,\frac{1}{3}\,\frac{9}{2})$ | $(0\,2\,\bar{3})$ | 130 | 1.65 | 220 |
| $(\frac{1}{3}\,\frac{1}{3}\,6)$ | $(0\,2\,\bar{4})$ | 73 | 1.92 | 220 |
| $(\frac{1}{3}\,\frac{1}{3}\,9)$ | $(0\,2\,\bar{6})$ | 58 | 2.47 | 220 |
| $(1\,0\,\bar{5})^a$ | $(1\,3\,3)$ | ∼300 | 2.45 | 190 |
| $(1\,0\,7)^a$ | $(1\,3\,\bar{5})$ | ∼300 | 2.73 | 190 |
| $(1\,1\,3)^a$ | $(0\,6\,\bar{2})$ | ∼80 | 3.73 | 190 |

$^a$magnetic contribution

TABLE VI: Possible spin structures for the high-$H$ phase obtained from our simulations explained in the text. Only half of the spins on the particular Fe sites according to Tab. III are presented. The other half is obtained by adding ($\frac{1}{2}\,\frac{1}{2}\,0$) with the same spin direction due to the still valid C-centering condition.

| high-$H$ solution ($\chi^2$) | Fe1 | Fe2 | Fe3 | Fe4 | Fe5 | Fe6 | Fe7 | Fe8 | Fe9 | Fe10 | Fe11 | Fe12 |
|---|---|---|---|---|---|---|---|---|---|---|---|---|
| 1 (2.05) | ↑ | ↓ | ↑ | ↓ | ↑ | ↑ | ↑ | ↑ | ↓ | ↓ | ↑ | ↑ |
| 2 (55.07) | ↓ | ↑ | 0 | ↑ | 0 | ↑ | ↓ | ↑ | 0 | ↑ | ↑ | ↓ |
| 3 (15.29) | ↓ | 0 | 0 | ↑ | ↓ | ↑ | ↓ | ↑ | 0 | ↑ | ↑ | ↓ |

## The spin structures and symmetry

A spin structure established in $H=0$ on a crystal with space group $C2/m$ would usually be expected to follow one of the four magnetic space groups $C2/m$, $C2/m'$, $C2'/m'$ and $C2'/m$ corresponding to one of four irreducible representations, according to which all crystallographic sites involved in spin order should order. For both spin structures established here this is not the case (even taking into account symmetry equivalent structures (i.e., a shifted cell) and both possible positions of the inversion center in the monoclinic cell), because the spins on different sites inevitably order according to different representations. In fact, requiring all sites to follow the same representation (or remain disordered) corresponds to only 40 different structures, the diffraction pattern of all of which is very obviously inconsistent with observation. Different irreducible representations on different sites are inconsistent with magnetic ordering occurring via a single second order phase transition [7]. In the case of $LuFe_2O_4$, the apparent degeneracy of two phases at $T=T_N$ and $H=0$ indeed makes a simple second-order transition unlikely.

---


[1] A. D. Christianson *et al.*, Phys. Rev. Lett. **100**, 107601 (2008).
[2] K.-T. Ko *et al.*, Phys. Rev. Lett. **103**, 207202 (2009).
[3] K. Kuepper *et al.*, Phys. Rev. B. **80**, 220409(R) (2009).
[4] X. S. Xu *et al.*, Phys. Rev. B. **82**, 014304 (2010).
[5] M. Angst *et al.*, Phys. Rev. Lett. **101**, 227601 (2008).
[6] N. Ikeda *et al.*, Nature **436**, 1136 (2005).
[7] See e.g., J.Rossat-Mignod in: 'Methods in Experimental Physics', ed. K. Sköld and D. L. Price (Academic Press, 1987).
